# Supplementary material for: Fast conformational clustering of extensive molecular dynamics simulation data
Source: arXiv:2301.04492 ancillary file (2023-01-11)
Supplement: Supplementary file 1 [file hunkler_peter_SI.pdf]

# Supporting Information:
# Fast conformational clustering of extensive molecular dynamics simulation data

Simon Hunkler,[1] Kay Diederichs,[1] Oleksandra Kukharenko,[2,*] and Christine Peter[1,†]

[1] *Department of Chemistry, University of Konstanz*

[2] *Theory Department, Max Planck Institute for Polymer Research*

(Dated: January 11, 2023)

## S-I. CHOICE OF THE PARAMETERS FOR THE PROPOSED SCHEME

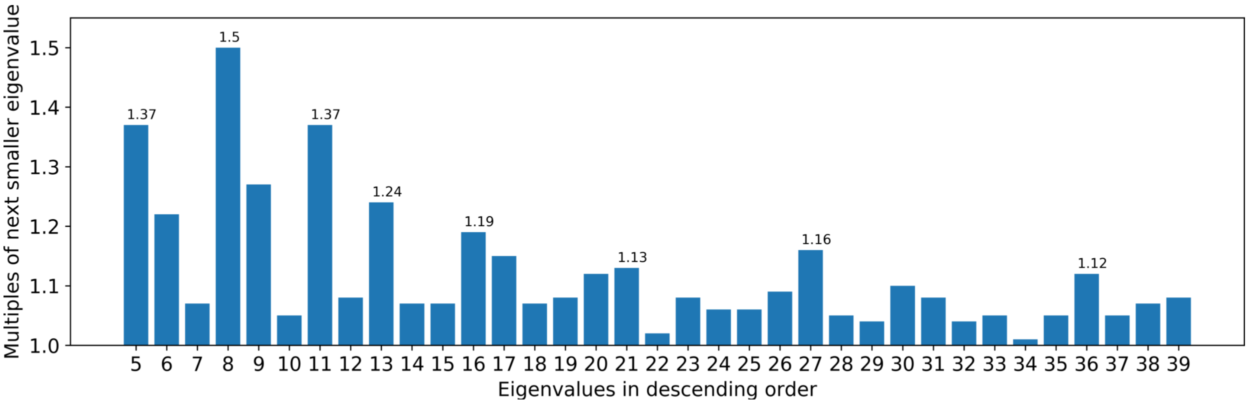


FIG. S1. Graph showing the comparison of one eigenvalue to the next one in multiples of the next eigenvalue. This example shows the Trp-cage eigenvalues from the 5th to the 39th strongest eigenvalue/eigenvector pair.

In order to decide how many dimensions the cc_analysis subspace should include, a plot like shown in Figure S1 can be used. It shows the comparison of one eigenvalue to the next one in multiples of the next eigenvalue, beginning with the 5th strongest eigenvalue/eigenvector pair. To find a spectral gap we compare the ratio between subsequent eigenvalues. Bars in Figure S1 correspond to the size of the gaps. One can use the height of

* kukharenko@mpip-mainz.mpg.de

† christine.peter@uni-konstanz.de

bars as an indication for the dimensionality to choose in the cc_analysis space. We selected few dimensions and performed a test-clustering.

In this test each of the subspaces that were selected based on the eigenvalue plot (in this example it could be 5, 8, 11, 13, 16, 21, 27 and 36 dimensions) are clustered using the HDBSCAN algorithm. The HDBSCAN parameters min_cluster_size and min_samples can be varied as well (e.g. 5, 10, 20, 40, 60, 80, 100, 120, 140, 160, 180, 200) and for each combination of dimensionality and HDBSCAN parameters a clustering is performed. Clustering results were then evaluated for each combination of dimensionality and clustering parameters by the internal cluster root-mean-square deviations (RMSDs) of the $C_\alpha$ atoms in the protein backbone. As a reference structure the central conformation of each cluster was used. This central conformation is identified as the structure with the lowest sum of the RMSDs to all other conformations in a given cluster. In order to compute the RMSDs a Python package called pyRMSD[S1] was used.

Once the RMSDs of all clusters are computed, an average RMSD value for all clusters of one dimensionality/HDBSCAN parameter combination can be obtained. The combination that gives the lowest average RMSD value is used for refining both the choice of the dimensionality as well as the HDBSCAN parameters. For the example from Figure S1 a combination of a 21 dimensional cc_analysis space and HDBSCAN parameters of 10 gave the lowest average RMSD out of the probed combinations. After some parameter refinement we ended up using a dimensionality of 20 and HDBSCAN parameters of 12 to cluster the first iteration of the Trp-cage system.

## S-II. STOPPING CRITERIA

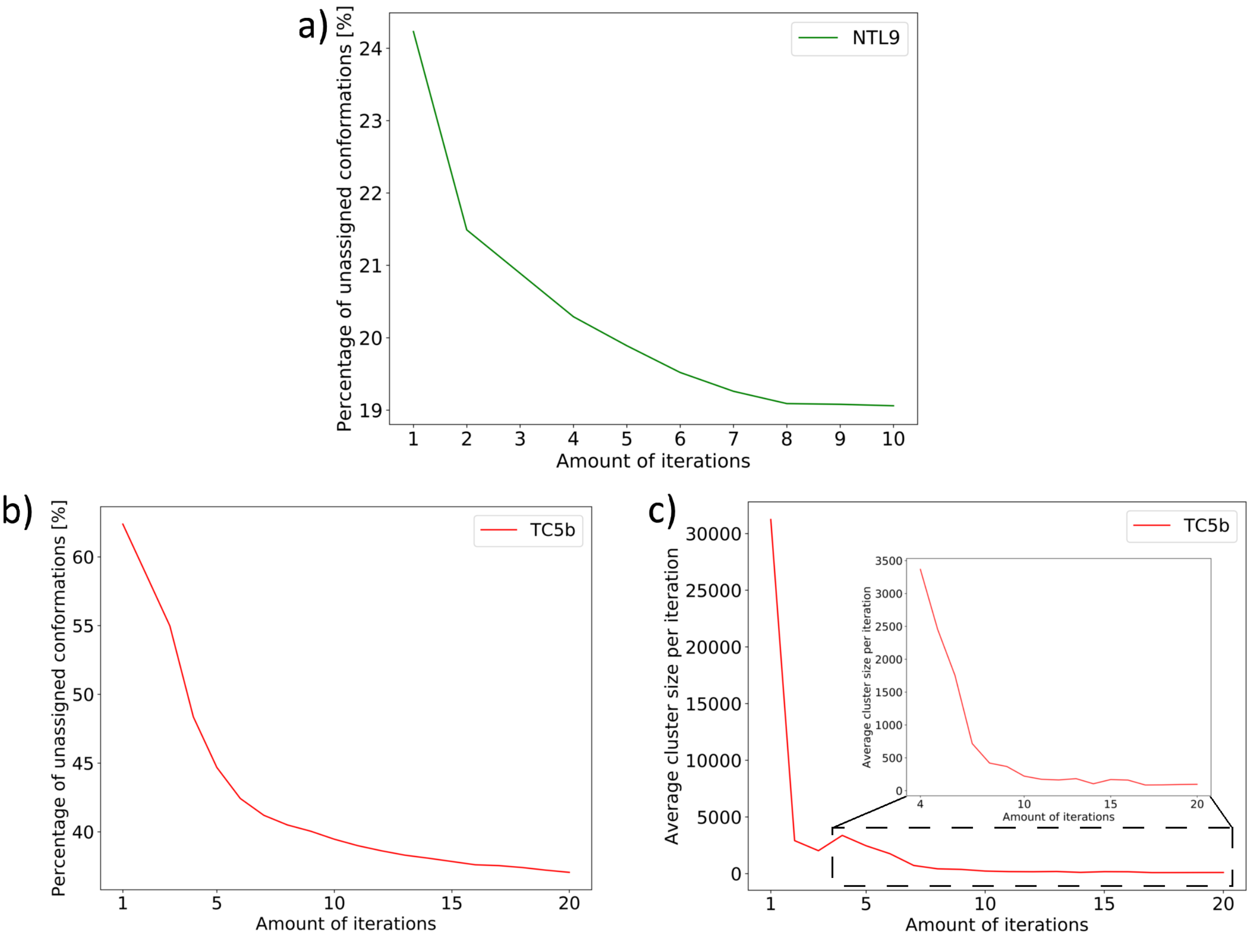


FIG. S2. Stopping criteria for the clustering workflow: monitoring the percentage of the unassigned data and the average cluster sizes after each iteration. (a) For the NTL9 system after the 8th iteration the curve starts to flatten and the clustering workflow could be stopped at this point. For TC5b no convergence in the number of clustered structures is observed even after 20 iterations (b), but the newly found clusters contain only few configurations (c) and the workflow could be stopped after about 8-10 iterations.

## S-III. RMSD PLOTS

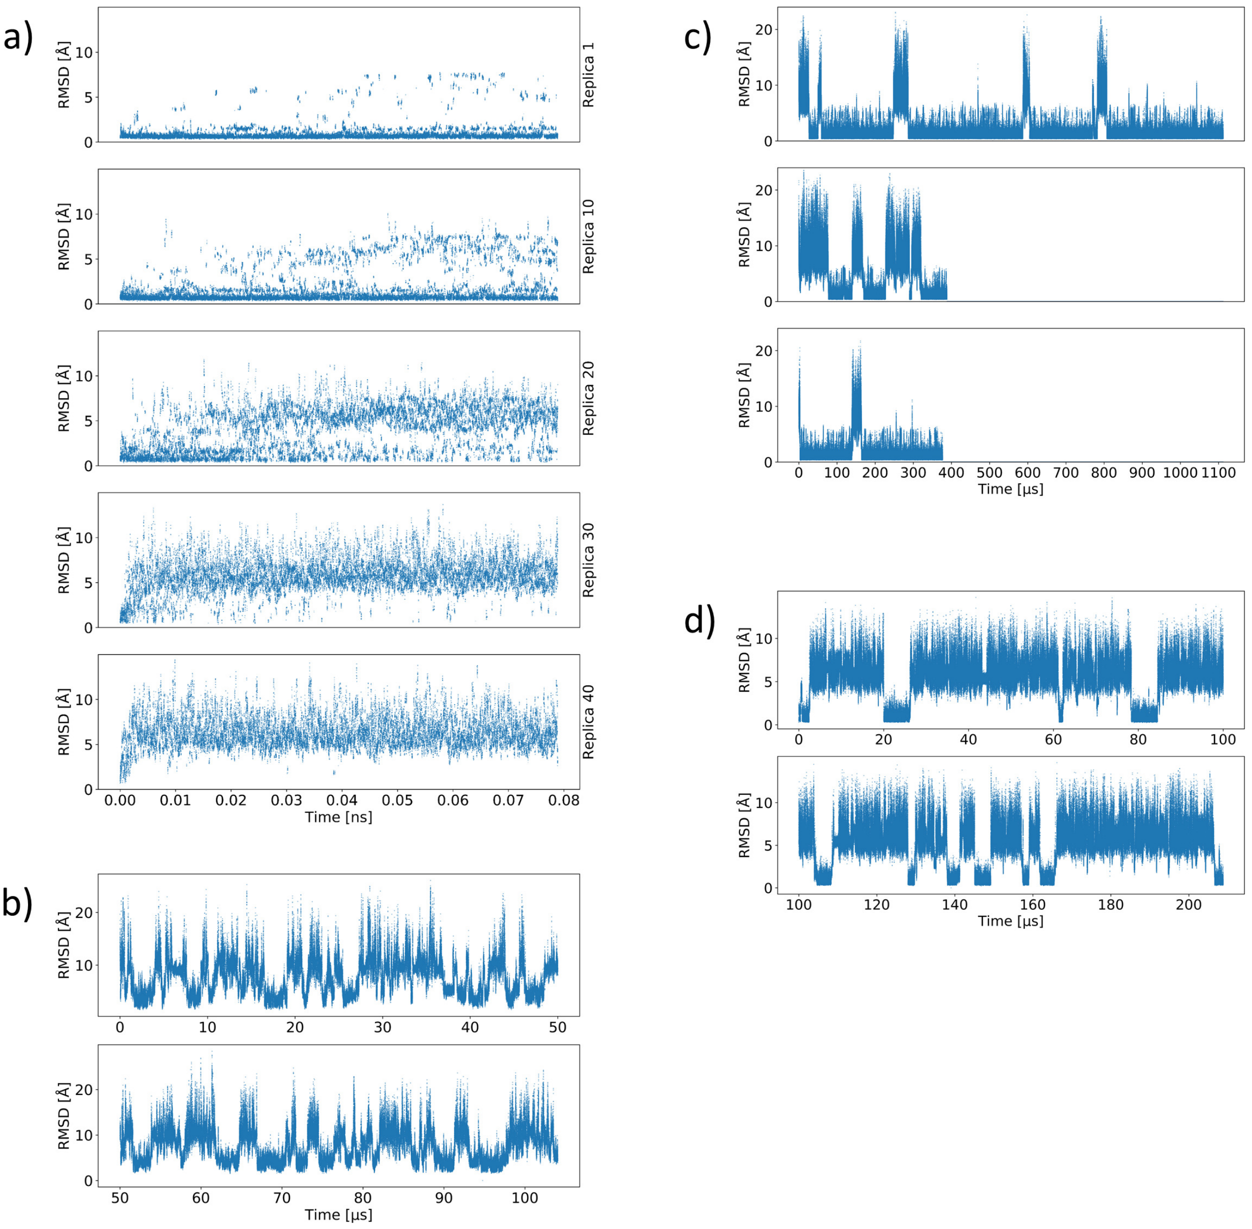


FIG. S3. RMSD plots compared to the experimental structure of the closest homologue for all four systems that were analysed in this article: a) Trp-cage RM (TC5b), b) Trp-cage Anton (TC10b), c) Protein B (1PRB) and d) NTL9 (2HBA).

## S-IV. K-MEANS CLUSTERING

We used principal component analysis (PCA) [S2, S3] on the pairwise $C_\alpha$ distances of the TC5b system and thereby generated a 11 dimensional PCA projection that represents

90% of the variance in the data. This PCA space was then used for clustering with the k-means algorithm [S4, S5]. We conducted the clustering twice, once by setting the number of clusters to 2500 and once to 25000 (k-means requires a pre-specification of the number of clusters).

In order to compare these clusterings in a fair way to our results we analysed only the

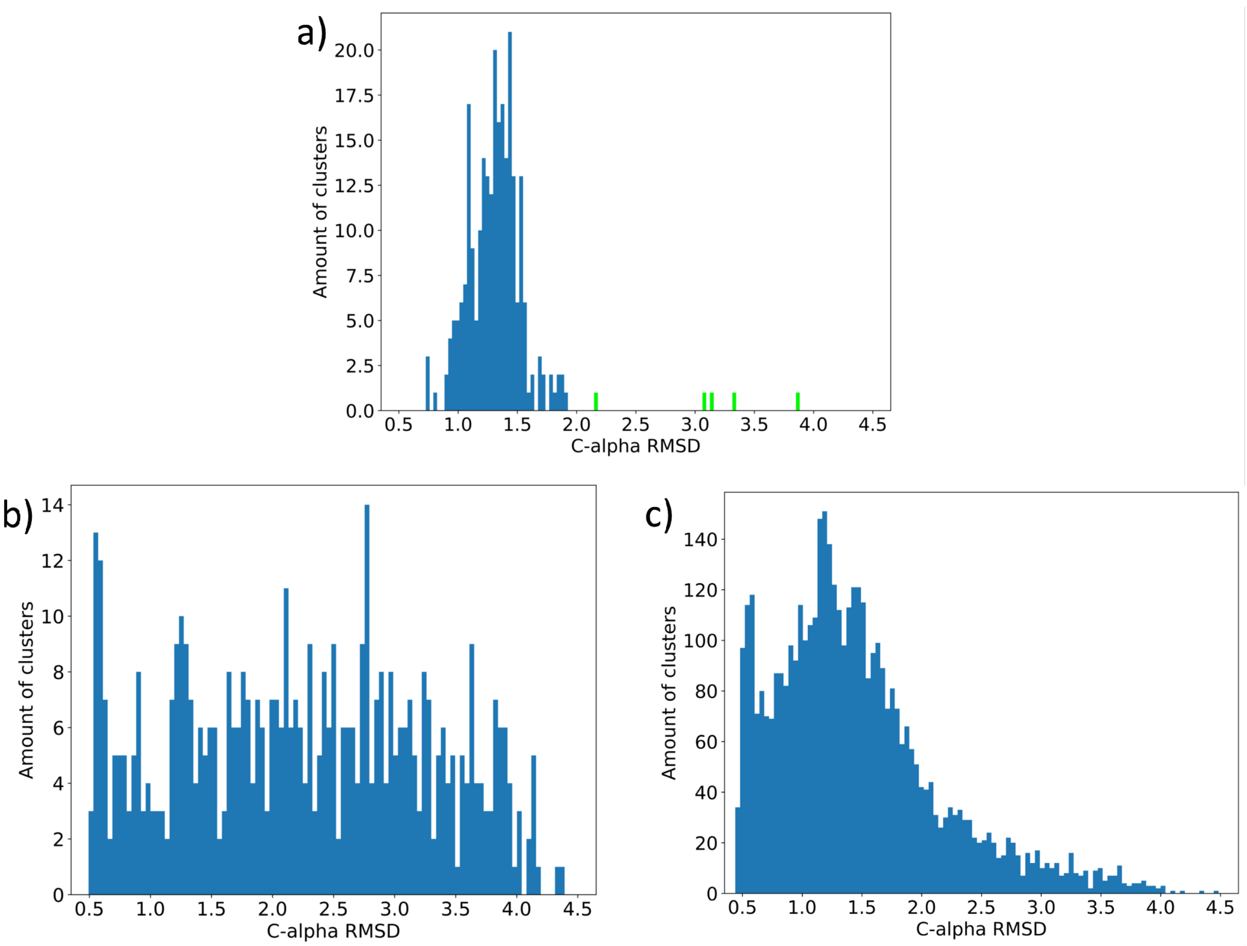


FIG. S4. Comparison of RMSD distributions in the clusters of TC5b obtained with the proposed scheme and the combination of PCA and k-means. (a) 260 clusters (contain 60.5% of the data) found during the 10 clustering iterations of the proposed clustering workflow. A RMSD cutoff is one of the parameters in our method. It was set to 1.8 Åfor most iterations (blue distribution). For one iteration it was increased to obtain fuzzy clusters that are not well defined but share a general structural motif (green bars). (b) The 526 biggest clusters obtained with k-means (out of k=2500 overall clusters) representing the same 60.5% of the data as the 260 clusters of our clustering workflow. (c) The biggest 4395 k-means clusters (k=25000) representing the same 60.5%.

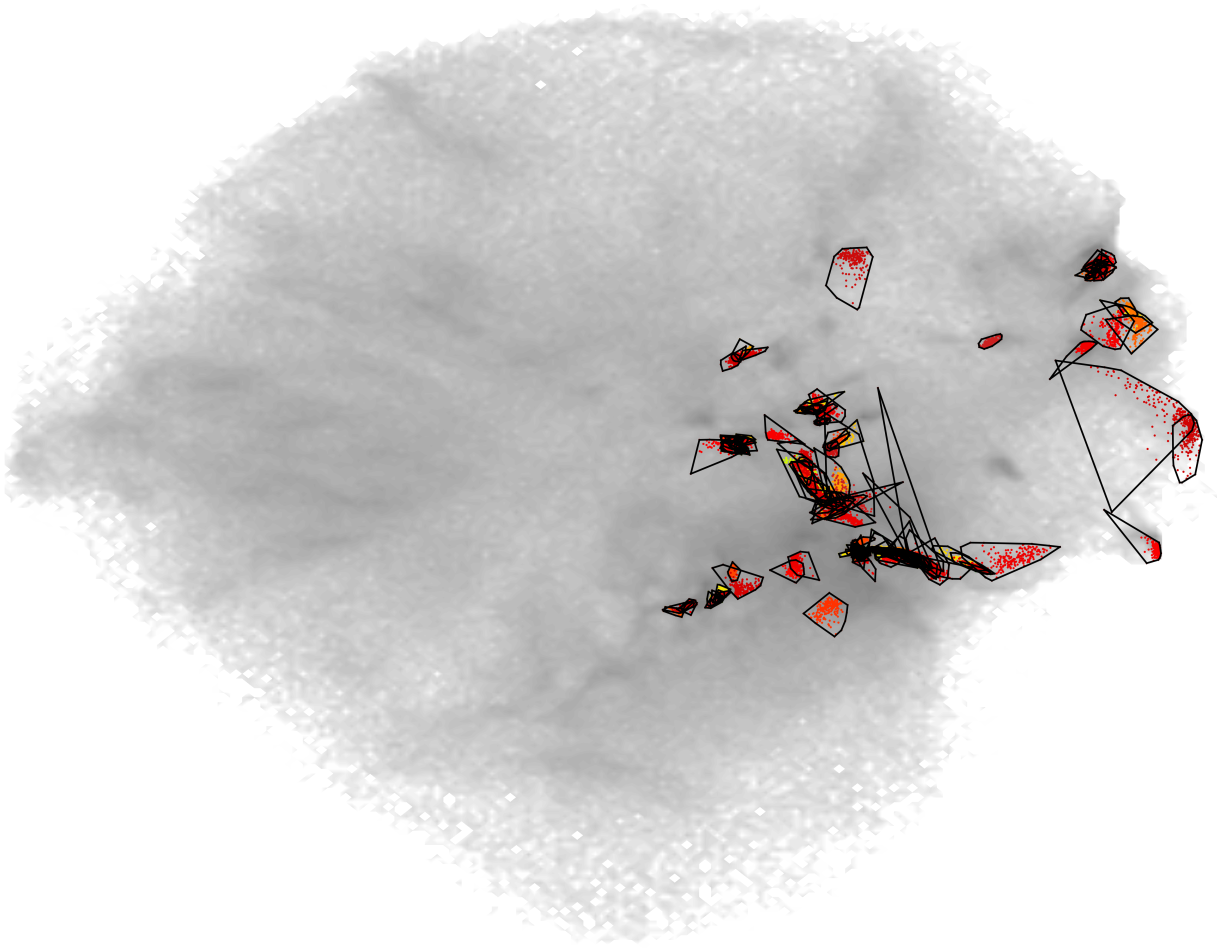

FIG. S5. The largest 1000 clusters found by applying k-means with 25000 cluster centers to a 11 dimensional PCA space projected to the same 2D encodermap space as we used for the clustering of the TC5b system (Figure 4 in the main text).

largest clusters that add up to 60.5% of the data, which is the amount of conformations that we assigned to clusters after 10 iterations of our clustering workflow. The average internal cluster RMSD distributions of these k-means clusterings (that represent 60.5% of the data) as well as of our clustering are shown in Figure S4. With our clustering workflow we represent 60.5% of the data in 260 clusters with an average internal cluster RMSD of 1.34 Å. The combination of PCA and k-means represents the same percentage of the data set in 526 and 4395 clusters with an average internal cluster RMSD of 2.24 Å and 1.46 Å for the 2500 and 25000 cluster centers, respectively. From these numbers it can be seen that only the clustering with 25000 clusters centers has a comparable average internal cluster

RMSD to our clustering. Moreover the RMSD distribution in Figure S4c shows that the k-means clustering needs to include a large amount of structurally undefined clusters in order to represent the same amount of data. Additionally the choice of the necessary amount of clusters and which percentage of them contains structurally similar configurations is not known a priory. Figure S5 shows the largest 1000 clusters of the k-means clustering (k=25000) projected to the encodermap space which we used for the clustering of the TC5b system (Figure 4 in the main text). The k-means clusters projected to this 2D map are very locally confined, which again shows that the 2D encodermap projection indeed separates different structures to different parts of the map very nicely. The clustering of such a large data set with 25000 cluster centers ran for about 23 hours on the local workstation compared to 2.5 hours for our clustering workflow.

## S-V. WORKSTATION SPECIFICATIONS

All analysis was performed on a standard workstation with the following specifications: CPU: Intel Xeon Gold 6126T with 24 threads, 2.6 GHz; RAM: 80 GB DDR4; GPU: NVIDIA GeForce GTX 1080 Ti

---

[S1] V. A. Gil and V. Guallar, pyRMSD: a Python package for efficient pairwise RMSD matrix calculation and handling, Bioinformatics **29**, 2363 (2013).

[S2] K. Pearson, Liii. on lines and planes of closest fit to systems of points in space, Philos. Mag. (1798-1977) **2**, 559 (1901).

[S3] H. Hotelling, Analysis of a complex of statistical variables into principal components., J. Educ. Psychol. **24**, 417 (1933).

[S4] J. B. MacQueen, Some methods for classification and analysis of multivariate observations, in Proc. of 5th Berkeley Symp. Math. Statist. Probability, Vol. 1, edited by L. M. L. Cam and J. Neyman (University of California Press, 1967) pp. 281–297.

[S5] D. Arthur and S. Vassilvitskii, K-means++: The advantages of careful seeding, in Proc. of 8 ACM-SIAM Symp. on Discrete Algorithms, SODA '07 (SIAM, Philadelphia, PA, USA, 2007) pp. 1027–1035.
